# Supplementary material for: Taming Diffusion Probabilistic Models for Character Control
Source: arXiv:2404.15121 source file (2024-04-23)
Supplement: Supplementary file 1 [file 7-appendix.tex]

% \section{Appendix}
% %%
% %%
% %% Bullet points
% %% 1.  how to build the pyramid
% %% 2.  dataset?
% %% 3.  hyper-parameters
% %%
\section{Effects of Hyper-parameters}
\label{hyperparameters}
% \wy{
% 1. how to deal with the K, patch size and r.
% 2. 
% }
Our framework involves several hyper-parameters during the synthesis process. 
In this section, we discuss the effects of these hyper-parameters. The quantitative results are presented in \Cref{tab:hyperparameters}.
% Table~\ref{tab:hyperparameters} presents the effect of different hyperparameters. 
%Although we provide the controls over them, we use the same the ·set of hyper-parameters, namely $K = ..., p = ..., r = ..., ...$ in all ours experiments unless otherwise specified.

\paragraph{Effects of $\alpha$}
As rarely-appearing patches have a larger minimal distance,
the completeness of the synthesis is encouraged by normalizing the distance of patches extracted from examples with their minimal distance to the initial guess. 
Therefore, the $\alpha$ in Equation 2 serves as a control knob for the completeness of exemplar patches in the synthesized result.
As it restricts the lower bound of the normalizing denominator, a smaller $\alpha$ value encourages more preservation of the example content in the synthesis.
As shown in Table~\ref{tab:hyperparameters}, when $\alpha$ decreases to a certain level, a higher coverage score is achieved. However, if the value $\alpha$ is too small, an excessive emphasis on completeness (especially for patches with almost zero distance to the generated motion) can overwhelm the similarity measure used for the matching process, resulting in unstable generation and low-quality motion (evidenced by low coverage and high patch distances of the corrupted results)."

\paragraph{Effects of $K$}
The ratio of the patch size to the length of input example motion at the coarsest stage 
controls the receptive field for synthesis, similar to the concept in image domain.
A larger $K$ causes a smaller receptive field, leading to more diverse results.
In particular,
a large $K$ allows only capturing fine-level movements and leads to some unnatural transitions, while a small $K$ leads to overfitting of the original sequence. 
Table~\ref{tab:hyperparameters} shows the global and local patch distance increase as $K$ increases. 
This is because the generated result deviates further from the input sequence when the receptive field is smaller.
% controls the diversity of the synthesized motion.

\paragraph{Effects of patch size $\patchsize$}
The patch size $\patchsize$ defines the temporal length of patches used in the generative matching and blending. 
Patch size controls the receptive field jointly with $K$, and a smaller patch size leads to a smaller receptive field, which creates less coherent result as shown by the increase of global and local patch distance in \Cref{tab:hyperparameters}.
% A larger $\patchsize$ encourages more coherent synthesized results 
% and this knob provides a large wide of flexibility which does not affect the quality too much.

\paragraph{Effects of $\downsamplef$}
The factor $\downsamplef$ controls the step size of transition between stages. A large step size, controlled by a large $\downsamplef$, may result in unstable generation due to big gaps between consecutive scales. On the other hand, a small step size causes unnecessary running time.

\begin{figure}[t!]
  \centering
  \includegraphics[width=\linewidth]{image/web_demo.pdf}
  \caption{Screenshot of our web interface. Characters in grey are synthesized.
  }
  \label{fig:webdemo}
\end{figure}

\begin{figure}[t!]
  \centering
  \includegraphics[width=\linewidth]{image/blender_addon.pdf}
  \caption{Screenshot of our Blender add-on. Left: The input animation. Right: Highlighted synthesized animation.
  }
  \label{fig:blenderaddon}
\end{figure}

\begin{table}[t!]
\caption{
The different settings of hyperparameters.
}
\footnotesize
\setlength{\tabcolsep}{1.5pt}
\centering

\begin{tabular}{lccccc} 
\toprule
 & Coverage & Set Diversity & Global Patch Dist. & Local Patch Dist. \\ 
\midrule
Ours (not use $\alpha$) & 87.45 & 0.27 & 0.18 & 0.17 \\
Ours ($\alpha = 5$) & 87.89 & 0.27 & 0.18 & 0.17 \\
Ours ($\alpha = 0.5$) & 88.47 & 0.27 & 0.18 & 0.17 \\
Ours ($\alpha = 0.05$) & 93.80 & 0.27 & 0.18 & 0.17 \\
Ours ($\alpha = 0.005$) & 99.96 & 0.27 & 0.30 & 0.23 \\ 
Ours ($\alpha = 0.0$) & 36.78 & 0.25 & 2.17 & 1.60 \\ 
\midrule
Ours ($K = 20$) & 87.74 & 0.25 & 1.03 & 0.71 \\
Ours ($K = 15$) & 92.04 & 0.26 & 0.73 & 0.54 \\
Ours ($K = 10$) & 96.07 & 0.27 & 0.42 & 0.36 \\
\midrule
Ours ($\patchsize = 23$) & 99.85 & 0.26 & 0.27 & 0.24 \\
Ours ($\patchsize = 17$) & 99.88 & 0.26 & 0.23 & 0.21 \\
Ours ($\patchsize = 5$) & 99.66 & 0.27 & 0.41 & 0.32 \\
\midrule
Ours ($\downsamplef = 2$) & 99.61 & 0.27 & 0.22 & 0.20 \\
Ours ($\downsamplef = 4$) & 99.16 & 0.27 & 0.34 & 0.28 \\
Ours ($\downsamplef = 8$) & 97.97 & 0.26 & 0.57 & 0.42 \\ 
\bottomrule
\end{tabular}

\label{tab:hyperparameters}
\end{table}%

\section{User Interface}
Our framework is general, lightweight, and easy to integrate into many production tools.
%
%% Web Demo
For novice users, we build a user-friendly website where users can upload their motion files and then synthesize diverse novel motions with a single click, as demonstrated in \Cref{fig:webdemo}.
%% Blender addon
We also develop a Blender add-on for professional artists, which seamlessly integrates into their existing workflow as demonstrated in \Cref{fig:blenderaddon}.
Note both of the interfaces runs efficiently on a consumer-level laptop. Please refer to the accompanying video for the results.
